# Supplementary material for: Learning solutions of parameterized stiff ODEs using Gaussian processes
Source: arXiv:2511.05990 source file (2025-11-08)
Supplement: Supplementary file 1 [file ODEGPS_supplement.pdf]

# SUPPLEMENTARY MATERIALS: LEARNING SOLUTIONS OF PARAMETERIZED STIFF ODES USING GAUSSIAN PROCESSES*

IDOIA CORTES GARCIA†, PETER FÖRSTER‡, WIL SCHILDERS§, AND SEBASTIAN SCHÖPS¶

**SM1. Examples.** In the following, we collect additional results for the examples from section 4. Figure SM1 shows the results for the non-stiff range of the VDPO ($p \in [0.5, 1.5]$), arranged in a similar fashion as Figure 8. We again observe similar behavior as in the one-dimensional case, in that the convergence rates remain almost unchanged between the conventional and reparameterized designs. The bottom right plot shows the reparameterized prediction based on the design with $\mu = 1$, providing a visual comparison with the reference from the top left of Figure 6.

Figure SM2 contains the results for the second solution component of the TDO. The corresponding reparameterized designs only show comparatively small improvements in the convergence rates, however this is again in line with the expectation when taking into account the corresponding MMRs. Table SM1 lists the MMRs for the second solution components of the TDO and Brusselator, analogous to Table 1. The tables indicate that the second solution component of the TDO behaves similar to the VDPO in the non-stiff range, implying that only a small improvement, if any, is expected from the reparameterization.

Finally, Figure SM3 shows the results for the second solution component of the Brusselator. In this case, we observe very similar rates as for the first component, compare Figure 10. This is once again in line with the expectations set by the MMRs, compare Table SM1 and Table 1.

*Submitted to the editors DATE.

**Funding:** This work is supported by the Graduate School CE within the Centre for Computational Engineering at Technische Universität Darmstadt and the ECSEL Joint Undertaking (JU) under grant agreement No. 101007319. The JU receives support from the European Union's Horizon 2020 research and innovation programme and the Netherlands, Hungary, France, Poland, Austria, Germany, Italy and Switzerland. Note that this work only reflects the authors' views and that the JU is not responsible for any use that may be made of the information it contains.

†Eindhoven University of Technology, Eindhoven, The Netherlands.

‡Technical University of Darmstadt, Darmstadt, Germany and Eindhoven University of Technology, Eindhoven, The Netherlands. (peter.foerster@tu-darmstadt.de).

§Eindhoven University of Technology, Eindhoven, The Netherlands.

¶Technical University of Darmstadt, Darmstadt, Germany.

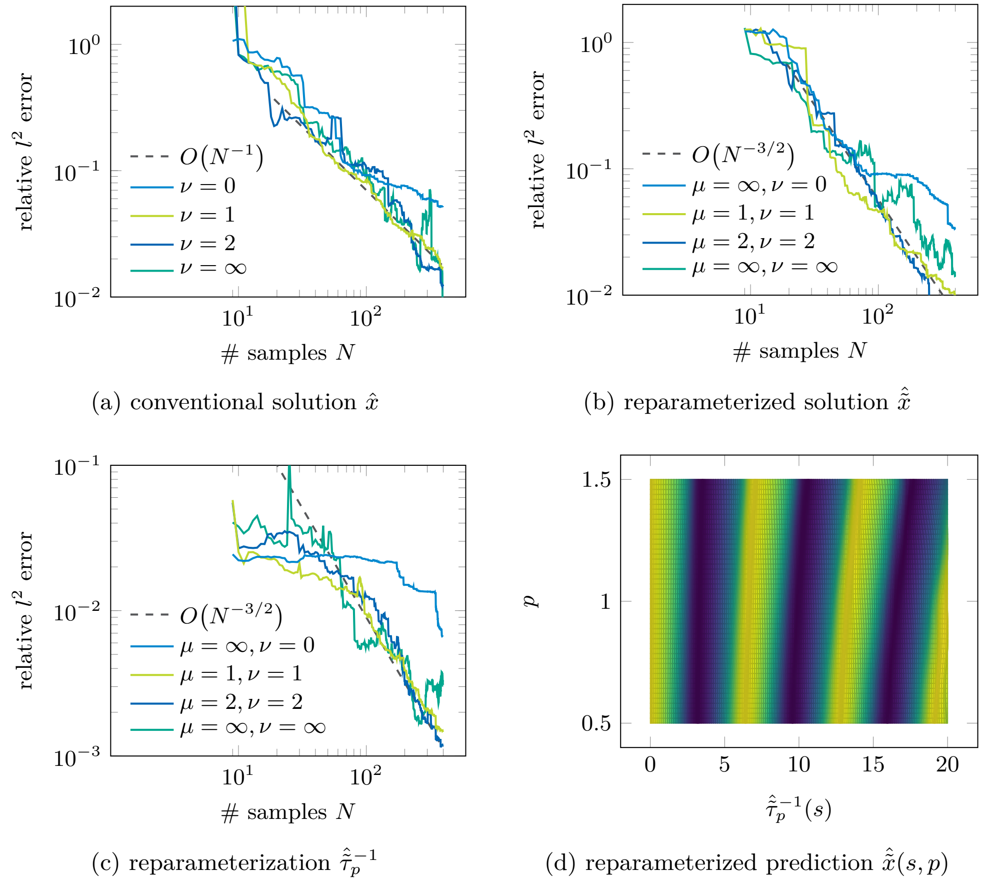


(a) conventional solution $\hat{x}$

(b) reparameterized solution $\hat{\tilde{x}}$

(c) reparameterization $\hat{\tilde{\tau}}_p^{-1}$

(d) reparameterized prediction $\hat{\tilde{x}}(s, p)$

Fig. SM1: Convergence results for conventional and reparameterized designs for the non-stiff parameter range of the VDPO. Reparameterized prediction based on the design with $\mu = 1$, compare the top left of Figure 6.

Table SM1: Factors of improvement in the convergence rates for the different examples, depending on the MMRs of the original solutions ($r$) and those of the reparameterized solutions ($\tilde{r}$) with $\mu = \infty$.

| example | $r$ | $\tilde{r}$ | factor |
|---|---|---|---|
| TDO ($x_2$) | 2.6 | 1 | 1-2 |
| Brusselator ($x_2$) | 10.7 | 1.7 | 2-3 |

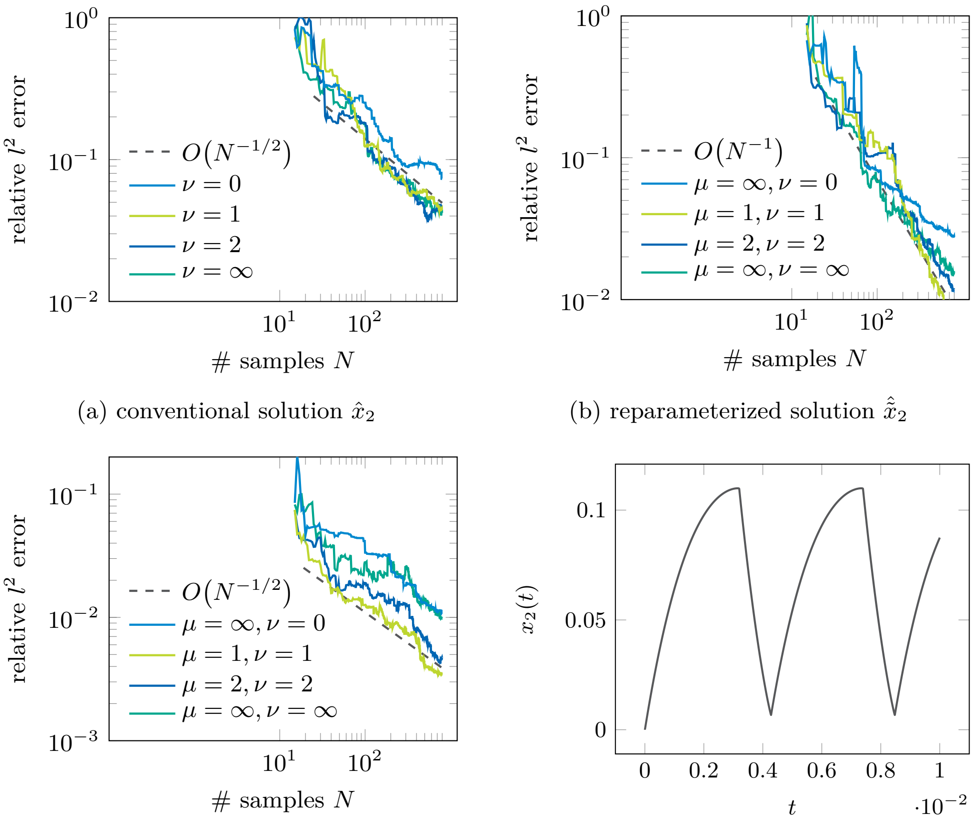


(a) conventional solution $\hat{x}_2$

(b) reparameterized solution $\hat{\tilde{x}}_2$

(c) reparameterization $\hat{\tilde{\tau}}_{\mathbf{p}}^{-1}$

(d) original solution $x_2$

Fig. SM2: Convergence results for conventional and reparameterized designs for the second solution component of the TDO. Original solution for $p_1 = 10^{-6}$, compare Figure 1 for the first component.

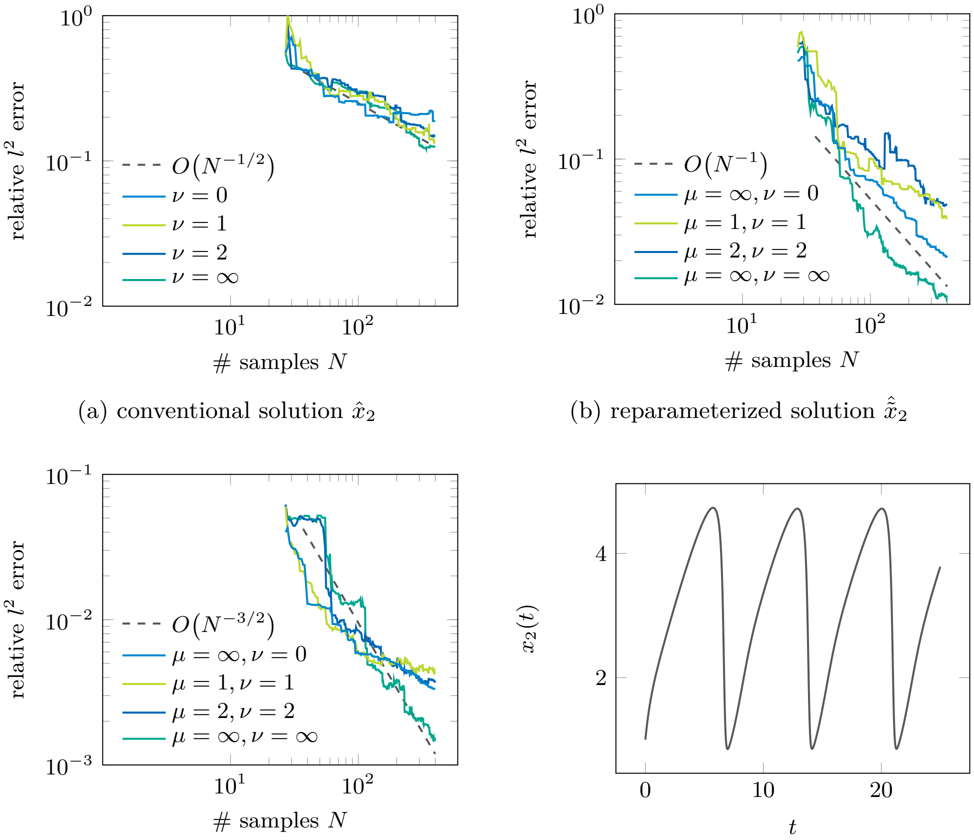


(a) conventional solution $\hat{x}_2$

(b) reparameterized solution $\hat{\tilde{x}}_2$

(c) reparameterization $\hat{\tilde{\tau}}_{\mathbf{p}}^{-1}$

(d) original solution $x_2$

Fig. SM3: Convergence results for conventional and reparameterized designs for the second solution component of the Brusselator. Original solution for $\mathbf{p} = [1, 3, 1, 1]^\top$.
